# Supplementary material for: Globally Interpretable Graph Learning via Distribution Matching
Source: arXiv:2306.10447 source file (2024-02-20)
Supplement: Supplementary file 1 [file appendix.tex]

\section{Appendix}

\subsection{GDM Algorithm}

\label{training_algo}
% \vskip 0.5em
% \noindent\textbf{Training Algorithm} 
To solve the final objective in Eq. (\ref{eq:final}), we use mini-batch based training procedure as depicted in Algorithm~\ref{alg}. 
We first initialize all the explanation graphs by sampling sub-graphs from the training graphs, with node number being set as the average node number of training graphs for the corresponding class.
The GNN model can be randomly initialized for $K$ times. For each randomly initialized GNN model, we train it for $T$ iterations. During each iteration, we sample a mini-batch of training graphs and explanation graphs. We first apply one step of update for explanation graphs based on the current GNN feature extractor; then update the GNN model for one step using normal graph classification loss.

\begin{algorithm}[h!]
 \caption{\ourmodel: Learning Explanation Graphs}
\label{alg}
\begin{algorithmic}[1]

\State \textbf{Input}: Training data $\mathcal{G}=\{\mathcal{G}_c\}^C_{c=1}$

\State Initialize explanation graphs $\mathcal{S}=\{\mathcal{S}_c\}_{c=1}^{C}$ for each class $c$

\For{$k=0,\dots,K-1$}
  
  \State Initialize GNN by sampling $\bm{\theta}_0\sim P_{\bm{\theta}}, \bm{\psi}_0 \sim P_{\bm{\psi}}$
  
  \For{$t=0,\ldots, T-1$}
      \State Sample mini-batch graphs $B^{\mathcal{S}}=\{B_c^{\mathcal{S}} \sim \mathcal{S}_c\}^C_{c=1}$ 

      \State Sample mini-batch graphs $B^{\mathcal{G}}=\{B_c^{\mathcal{G}} \sim \mathcal{G}_c\}^C_{c=1}$ 
    
    \State {\color{magenta}\textit{\# Optimize global interpretive graphs}}
    \For{class $c=1,\dots, C$}
    
      \State Compute the interpretation loss following Eq. (\ref{eq:final}): $\mathcal{L}_c=\mathcal{L}_\text{DM}(f_{\bm{\theta}_t}(B_c^{\mathcal{S}})) + \alpha\cdot\mathcal{L}_\text{feat}(B^{\mathcal{S}}_c) + \beta\cdot\mathcal{L}_\text{sparsity}(B^{\mathcal{S}}_c)$
    \EndFor
    \State Update explanation graphs $\mathcal{S} \leftarrow \mathcal{S} - \eta\nabla_{\mathcal{S}}\sum_{c=1}^{C}\mathcal{L}_c$

    \State {\color{magenta}\textit{\# Optimize GNN model as normal}}
    \State Compute normal training loss for graph classification task $\mathcal{L}_\text{CE}(h_{\bm{\psi}_{t-1}}, f_{\bm{\theta}_{t-1}})=\sum_{G\sim B^{\mathcal{G}}}\mathscr{l}(h_{\bm{\psi}_{t-1}}(f_{\bm{\theta}_{t-1}}(G)), y)$

    \State Update  $\bm{\theta}_{t+1}=\bm{\theta}_{t}-\eta_1\nabla_{\bm{\theta}}\mathcal{L}_\text{CE}(h_{\bm{\psi}_{t-1}}, f_{\bm{\theta}_{t-1}})$
    
    \State Update $\bm{\psi}_{t+1}=\bm{\psi}_{t}-\eta_2\nabla_{\bm{\psi}}\mathcal{L}_\text{CE}(h_{\bm{\psi}_{t-1}}, f_{\bm{\psi}_{t-1}})$
  \EndFor
\EndFor
\State \textbf{Output}: Explanation graphs $\mathcal{S}^*=\{\mathcal{S}^*_c\}_{c=1}^{C}$ for each class $c$
\end{algorithmic}
\end{algorithm}

\subsection{{Dataset Statistics}}
\label{sec:dataset}
The data statistics on both synthetic and real-world datasets for graph classification are provided in 
Table~\ref{summary_stats}. The ground-truth performance of GCN model is also listed for reference.

\begin{table}[h]
\centering
% \small
\caption{Basic Graph Statistics}
\begin{tabular}{lcccccc}
\toprule
 Dataset & \textbf{BA-Motif}  & \textbf{BA-LRP}  & \textbf{Shape} & \textbf{MUTAG} & \textbf{Graph-Twitter} & \textbf{Graph-SST5}   \\
 \midrule
 \# of classes & 2 & 2 &  4 & 2 & 3 & 5\\ 
 % \midrule
 \# of graphs & 1000 & 20000 & 100 & 188 & 4998 & 8544\\
 Avg. \# of nodes & 25 & 20 & 53.39 & 17.93  & 21.10 & 19.85\\
 % \midrule
 Avg. \# of edge & 50.93 & 42.04 &813.93 & 19.79  & 40.28 & 37.78\\
 \midrule
 GCN Accuracy & 100.00 & 97.95 & 100.00 & 88.63& 61.40 & 44.39\\
\bottomrule
\end{tabular}
\label{summary_stats}
\end{table}

\subsection{\ourmodel{} versus Inherently Global-Interpretable Model}
\label{LR}

We compare the performance of \ourmodel with a simple yet inherently global-interpretable method, logistic regression with hand-crafted graph-based features. When performing LR on these graph-structured data, we leverage the Laplacian matrix as graph features: we first sort row/column of adjacency matrix by nodes' degree to align the feature dimensions across different graphs; we then flatten the reordered laplacian matrix as input for LR model. When generating interpretations, we first train a LR on training graphs and obtain interpretations as the top most important features (i.e. edges on graph) based on regression weights where average number of edges. We then report the utility of LR interpretations, shown in the following table \ref{tab:LR}. 

\begin{table}[h!]
\centering
\small
\caption{Utility of Logistic Regression}
\begin{tabular}{lcccccc}
\toprule
Dataset &MUTAG& BA-Motif&BA-LRP	&Shape&Graph-Twitter&Graph-SST5\\
 \midrule
LR Interpretation & 93.33\%	& 100\%&100\%&100\%&42.10\%&22.68\%\\
Original LR	&96.66\%	& 100\%&100\%	& 100\%& 52.06\%& 27.45\%\\
\bottomrule
\end{tabular}
\label{tab:LR}
\end{table}

\begin{table}[h!]
\centering
\small
\caption{Utility of \ourmodel on large datasets}
\begin{tabular}{lcccc}
\toprule
\# of interpretive graphs per class& Graph-Twitter& Graph-SST5\\
 \midrule
10	&56.43 $\pm$ 1.39	&40.30 $\pm$ 1.27\\
50	&58.93 $\pm$ 1.29	&42.70 $\pm$ 1.10\\
100	&59.51 $\pm$ 0.31	&44.37 $\pm$ 0.28\\
Original GCN Accuracy	& 61.40 & 44.39\\
\bottomrule
\end{tabular}
\label{tab:GDM_LARGE}
\end{table}

LR shows good interpretation utility on simple datasets like BA-Motif and BA-LRP, but it has much worse performance on more sophisticated datasets, compared with \ourmodel in table \ref{tab:GDM_LARGE}. For example, interpretations generated by \ourmodel can achieve close accuracy as the original GCN model.
% One important difference between our method and interpretable LR is that we provide model-level interpretation, thus we only generate a few (e.g. 10, 50, 100 per class) graphs as interpretations; while LR generates local interpretations with the same size of training data.

\subsection{\ourmodel{} versus Local Interpretation}
\label{sec:local-global}

As aforementioned, \ourmodel{} provides global interpretation, which is significantly different from the extensively studied local interpretation methods: we only generate few small interpretive graphs per class to reflect the high-level discriminative patterns the model captures; while local interpretation is for each graph instance. Though our global interpretation is not directly comparable with existing local interpretation, we still compare their interpretation utility to demonstrate the efficacy of our \ourmodel{} when we only generate a few interpretive graphs. The results can be found in Table \ref{tab:GDM_LOCAL_Utility}. We compare our model with GNNExplainer\footnote[1]{https://github.com/RexYing/gnn-model-explainer},PGExplainer\footnote[2]{https://github.com/flyingdoog/PGExplainer} and Captum\footnote[3]{https://github.com/pytorch/captum} on utility. 
For Graph-SST5 and Graph-Twitter, we generate 100 graphs for each class and 10 graphs for other datasets.

\begin{table}[h!]
\centering
\small
\caption{Utility Compared with Local Interpretation}
\resizebox{\columnwidth}{!}{%
\begin{tabular}{lccccccc}
\toprule

Datasets & \textbf{Graph-SST5} &  \textbf{Graph-Twitter}  & \textbf{MUTAG} & \textbf{BA-Motif} & \textbf{Shape} & \textbf{BA-LRP} & \\
\ourmodel{}& \textbf{44.43  $\pm$0.45}	& \textbf{59.51 $\pm$ 0.31}	&82.45$\pm$2 .48	&\textbf{98.00$\pm$0.00}	&\textbf{100 $\pm$0.00}	& \textbf{94.90$\pm$1.09}\\

GNNExplainer & 43.00$\pm$0.07 &	58.12$\pm$1.48 & 73.68$\pm$5.31 &	93.2$\pm$0.89	& 89.00$\pm$4.89&58.65$\pm$4.78 \\

PGExplainer&28.41 $\pm$ 0.00	& 55.46 $\pm$	0.03 & 75.62$\pm$4.68	& 62.58$\pm$0.66	& 71.75$\pm$1.85	& 50.25$\pm$0.15 & \\

Captum& 28.83$\pm$0.05	& 55.76$\pm$0.42	& \textbf{89.20$\pm$0.01} &	52.00$\pm$0.60	& 80.00$\pm$0.01	& 49.25$\pm$0.01 \\

\end{tabular}
}
\label{tab:GDM_LOCAL_Utility}
\end{table}

% \begin{table}[t!]
% \centering
% \small
% \caption{Fidelity Compared with Local Interpretation}
% \resizebox{\columnwidth}{!}{%
% \begin{tabular}{lccccccc}
% \toprule

% Datasets & \textbf{Graph-SST5} &  \textbf{Graph-Twitter}  & \textbf{MUTAG} & \textbf{BA-Motif} & \textbf{Shape} & \textbf{BA-LRP} & \\
% \ourmodel{}& 90.67$\pm$0.019 &	94.44$\pm$0.015	&96.67$\pm$0.045&95.00$\pm$1.11	&100.00$\pm$0.00&	96.67$\pm$0.023\\

% GNNExplainer & 100.00$\pm$0.00 &	100.00$\pm$0.00	& 93.20$\pm$1.12	& 100.00$\pm$0.00	&100.00$\pm$0.00 &	100.00$\pm$0.00 \\

% PGExplainer&100.00$\pm$0.00&	100.00$\pm$0.00	& 93.75$\pm$1.00	& 100.00$\pm$0.00	& 100.00$\pm$0.00& 	100.00$\pm$0.00
%  \\

% Captum& 100.00$\pm$0.00	& 100.00$\pm$0.00	& 89.47$\pm$0.02	& 100.00$\pm$0.00	& 100.00$\pm$0.00& 	100.00$\pm$0.00
%  \\

% \end{tabular}
% }
% \label{tab:GDM_LOCAL_Fidelity}
% \end{table}

Comparing these results, we can observe that the \ourmodel{} obtains higher utility score compared to different GNN explaination methods, with relatively small variance. 
% And for fidelity, \ourmodel{} has the highest score for MUTAG and Shape dataset while the performance does not degrade a lot on other datasets.

\subsection{One Use Case of In-Process Interpretation}
\label{OO}

A use case of in-process interpretation is when the queried data is very different from the data used to train the model (i.e. out-of-distribution): fidelity score could fail to reflect intrinsic patterns learned by the model, as post-hoc interpretation also heavily relies on the property of queried data; and post-hoc methods are usually used when only given the pre-trained model without knowing the training data (the scenario when training data is provided can be found in Appendix \ref{sec:local-global}). In contrast, our in-process interpretation is generated during model training without accessing any auxiliary data, and thus is free of influence from the quality of queried data.

To mimic such a out-of-distribution case, we conduct a post-hoc interpretation experiment where the GCN model is trained on BA-LRP, and is used on BA-Motif. We use PGExplainer as an example post-hoc (local) interpretation method. The post-hoc interpretation utility is shown below when training and test data are from the same or different distribution.

\begin{figure}[h!]
  \centering
  \includegraphics[width=\linewidth]{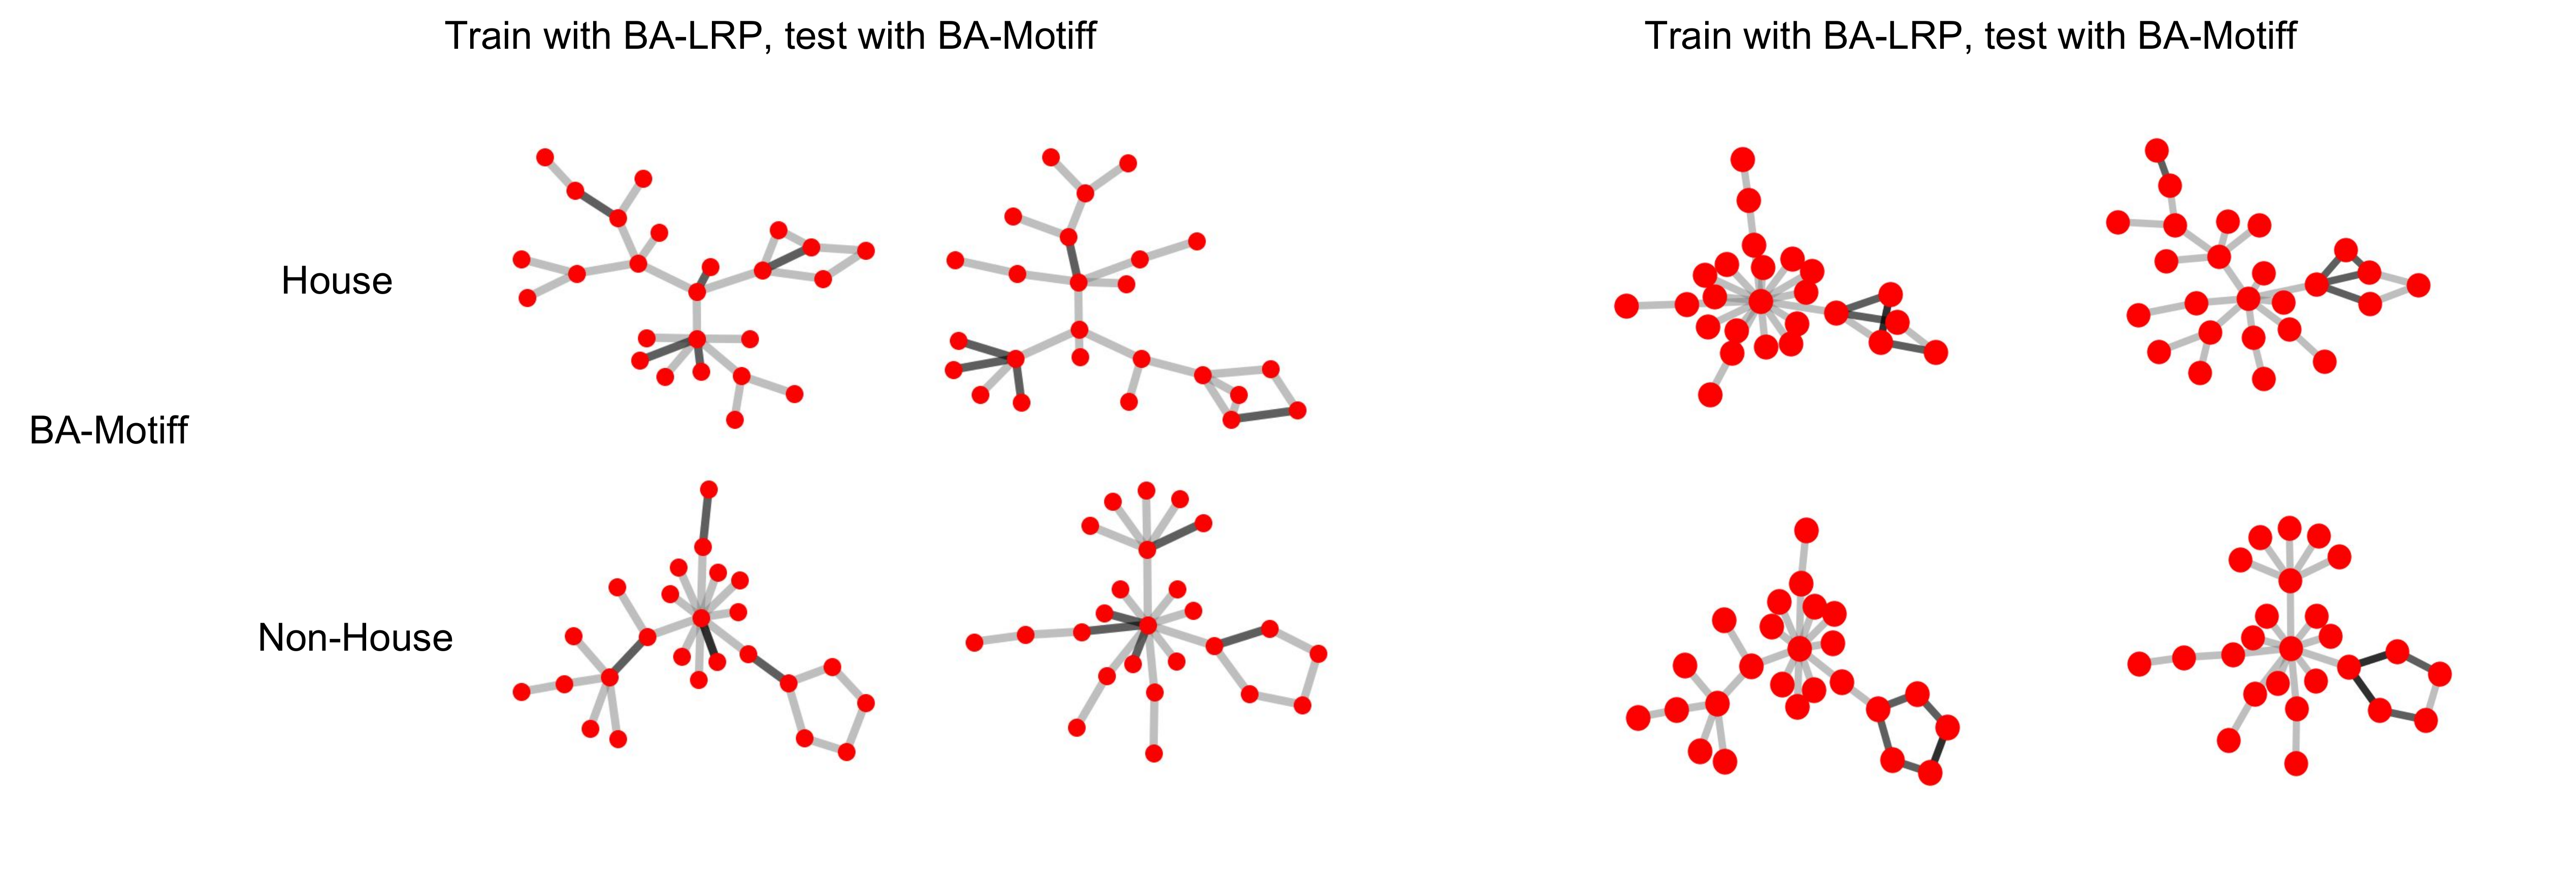}
\caption{Performance of PGExplainer under Out-of-distribution Scenario}
  \label{fig:oo}
\end{figure}

\begin{table}[h!]
\centering
\small
\caption{PGExplainer interpretation utility}
\begin{tabular}{cccc}
\toprule

Scenario & Training Data & Test Data & Utility $\pm$ std \\
\midrule
Same Distribution & BA-Motif & BA-Motif & 80.11 $\pm$ 0.08 \\
% \midrule
Out of Distribution & BA-LRP& BA-Motif & 75.34 $\pm$ 0.16\\
\bottomrule
\end{tabular}
\label{tab:oo}
\end{table}

As we expected, the utility drops 5\%. Meanwhile, we provide a visualization of generated interpretation via \ref{fig:oo} where we can see that PGExplainer fails to capture the most important motif in BA-Motif graphs (i.e. house/non-house subgraph). This case study demonstrates that post-hoc methods cannot provide valid interpretations under distribution shifts. In contrast, in-process interpretation is generated along with model training and does not rely on what instances are queried post-hoc. The out-of-distribution case could be popular in real-world scenarios, and in-process interpretation is a complementary tool for model interpretability when post-hoc interpretability is not possible/suitable.

\subsection{Hyperparameter Analysis}

\label{hyper-para}

In our final objective Eq. (\ref{eq:final}), we defined two hyper-parameters $\alpha$ and $\beta$ to control the strength for feature matching and sparsity matching regularization, respectively.

In this subsection, we explore the sensitivity of hyper-parameters $\alpha$ and $\beta$. Since MUTAG is the only dataset that contains node features, we only apply the feature matching regularization on this dataset. We report the in-process utility with different feature-matching coefficients $\alpha$ in Table \ref{tab:alpha}. A larger $\alpha$ means we have a stronger restriction on the node feature distribution. We found that when we have more strict restrictions, the utility increases slightly. This is an expected behavior since the node features from the original MUTAG graphs contain rich information for classifications, and matching the feature distribution enables the interpretation to capture rare node types. By having such restrictions, we successfully keep the important feature information in our interpretive graphs. 

\begin{figure}[h!]
  \centering
  \includegraphics[width=0.4\linewidth]{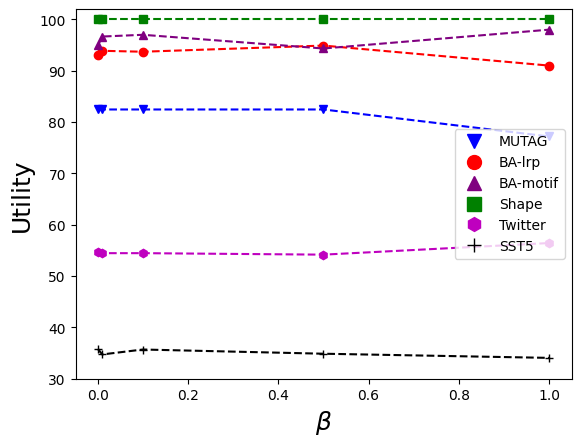}
\caption{Sensitivity analysis of hyper-parameter $\beta$ for the sparsity matching regularization}
  \label{fig:beta}
\end{figure}

Moreover, we vary the sparsity coefficient $\beta$ in the range of $\{0.001,0.01,0.1,0.5,1\}$, and report the utility for all of our four datasets in Figure \ref{fig:beta}. For most datasets excluding Shape, the performance start to degrade when the $\beta$ becomes larger than 0.5. This means that when the interpretive graph becomes more sparse, it will lose some information during training time.

\begin{table}[h!]
\centering
\small
\caption{Sensitivity analysis of hyper-parameter $\alpha$ for feature matching regularization. }
\begin{tabular}{lccccc}
\toprule
 $\alpha$ & 0.005  & 0.01 & 0.05& 0.5 & 1.0\\ [0.5ex] 
 \midrule
 Utility & 82.45 & 82.45 & 82.45 & 82.45 & 80.70 \\ 
\bottomrule
\end{tabular}
\label{tab:alpha}
\end{table}

\subsection{Special Case of Our Framework}

\label{no_update}
We also explore a special case when the GNN model is not updated when generating explanations, as discussed in Section~\ref{sec:final}. For this case, we randomly initialized different GNNs in each iteration with parameters fixed within each iteration as shown in algorithm \ref{alg:noupdate} To our surprise, the generated graphs are also quite effective in training a well-performed GNN. As shown in Table \ref{tab:train-time-init}, the interpretation utility of our methods does not degrade when the explanations are optimized without updating the GNN model in each iteration. This indicates that  randomly initialized GNNs are already able to produce informative interpretation patterns.
This finding echoes the observations from previous work in image classification~\cite{amid2022learning} and node classification~\cite{velickovic2019deep}. They have shown a similar observation that random neural networks can generate powerful representations, and random networks can perform a distance-preserving embedding of the data to make smaller distances between samples of the same class~\cite{giryes2016deep}.
Our finding further verifies such a property also stands for GNNs on the graph classification task from the perspective of model interpretation.

\begin{table}[h!]
\centering
\small
\caption{Utility without updating GCN.}
\begin{tabular}{lccccc}
\toprule
% \begin{tabular}[c]{@{}l@{}} \# of explanation \\ graph per class \end{tabular} 
Graphs/Cls & \textbf{BA-Motif} &  \textbf{BA-LRP}  & \textbf{Shape} & \textbf{MUTAG}  \\
\midrule
1 & 83.12 $\pm$ 2.16 & 79.95 $\pm$ 3.50  &  70.00 $\pm$ 21.60 & 71.93 $\pm$ 8.94 \\
5 &  99.33 $\pm$ 0.47 &  88.46 $\pm$ 1.11  & 100.00 $\pm$ 0.00 &89.47 $\pm$ 7.44 \\
10 & 100.00 $\pm$ 0.00 & 93.53 $\pm$ 3.41  & 100.00 $\pm$ 0.00 & 85.96 $\pm$ 2.48\\
\bottomrule
Graphs/Cls &  \multicolumn{2}{c}{\textbf{Graph-Twitter}}&  \multicolumn{2}{c}{\textbf{Graph-SST5}}   \\
\midrule
10 &  \multicolumn{2}{c}{52.97 $\pm$ 0.29}   & \multicolumn{2}{c}{40.30 $\pm$ 1.27}\\
50 &  \multicolumn{2}{c}{57.63 $\pm$ 0.92}  & \multicolumn{2}{c}{42.70 $\pm$ 1.10}\\
100 &  \multicolumn{2}{c}{58.35 $\pm$ 1.32} & \multicolumn{2}{c}{44.37 $\pm$ 0.28}\\
\bottomrule

\end{tabular}
\label{tab:train-time-init}
\end{table}

\begin{algorithm}[h!]
 \caption{GDM without GNN training}
\label{alg:noupdate}
\begin{algorithmic}[1]

\State \textbf{Input}: Training data $\mathcal{G}=\{\mathcal{G}_c\}^C_{c=1}$

\State Initialize explanation graphs $\mathcal{S}=\{\mathcal{S}_c\}_{c=1}^{C}$ for each class $c$

\For{$k=0,\dots,K-1$}
  
  \State Initialize GNN by sampling $\bm{\theta}_0\sim P_{\bm{\theta}}, \bm{\psi}_0 \sim P_{\bm{\psi}}$
  
  \For{$t=0,\ldots, T-1$}
      \State Sample mini-batch graphs $B^{\mathcal{S}}=\{B_c^{\mathcal{S}} \sim \mathcal{S}_c\}^C_{c=1}$ 

      \State Sample mini-batch graphs $B^{\mathcal{G}}=\{B_c^{\mathcal{G}} \sim \mathcal{G}_c\}^C_{c=1}$ 
      
    \For{class $c=1,\dots, C$}
    
      \State Compute the interpretation loss: \\$\mathcal{L}_c=\mathcal{L}_\text{DM}(f_{\bm{\theta}_L}(B_c^{\mathcal{S}})) + \alpha\cdot\mathcal{L}_\text{feat}(B^{\mathcal{S}}_c) + \beta\cdot\mathcal{L}_\text{sparsity}(B^{\mathcal{S}}_c)$
    \EndFor
    \State Update explanation graphs $\mathcal{S} \leftarrow \mathcal{S} - \eta\nabla_{\mathcal{S}}\sum_{c=1}^{C}\mathcal{L}_c$
    
  \EndFor
\EndFor
\State \textbf{Output}: Explanation graphs $\mathcal{S}^*=\{\mathcal{S}^*_c\}_{c=1}^{C}$ for each class $c$
\end{algorithmic}
\end{algorithm}

\subsection{Gain of Distribution Matching}
\label{sec:dm}

We construct an ablation method that adopts Algorithm \ref{alg} but replaces the design of matching embedding by matching the output probability distribution in the label space instead. The in-process utility of such a label-matching baseline is as follows in table \ref{tab:label-matching}:

\begin{table*}[h!]
\centering
% \small
\caption{Utility comparison, with a varying number of explanation graphs generated per class.}

\resizebox{\columnwidth}{!}{%
\begin{tabular}{lccccccc}
\toprule

\multirow{2}{*}{Graphs/Cls} & \multicolumn{3}{c}{\textbf{Graph-Twitter}} & \multicolumn{3}{c}{\textbf{Graph-SST5}}  \\
\cmidrule(rl){2-4}\cmidrule(rl){5-7}

 & \ourmodel{} & \ourmodel{}-label & Random & \ourmodel{} & \ourmodel{}-label & Random & \\
\midrule
10 & \textbf{56.43 $\pm$ 1.39}  & 40.00 $\pm$ 3.98 & 52.40 $\pm$ 0.29 &  \textbf{35.72 $\pm$ 0.65} & 25.49  $\pm$ 0.39 & 24.90 $\pm$ 0.60 \\
50 & \textbf{58.93 $\pm$ 1.29} & 55.62 $\pm$ 1.12 & 52.92 $\pm$  0.27&   \textbf{43.81 $\pm$ 0.86} & 31.47 $\pm$ 2.58  & 23.15 $\pm$ 0.35\\

100 &  \textbf{59.51 $\pm$ 0.31} & 53.37 $\pm$ 0.55 &  55.47 $\pm$ 0.51 &  \textbf{44.43  $\pm$ 0.45} & 32.01 $\pm$ 1.90  & 25.26 $\pm$ 0.75  \\

 & \multicolumn{3}{c}{\textbf{BA-Motif}} & \multicolumn{3}{c}{\textbf{BA-LRP}}  \\
\cmidrule(rl){2-4}\cmidrule(rl){5-7}

 & \ourmodel{} & \ourmodel{}-label & Random & \ourmodel{} & \ourmodel{}-label & Random & \\
\midrule
1 &  \textbf{71.66 $\pm$ 2.49}  & 50.63 $\pm$ 0.42 & 67.60 $\pm$ 4.52 & 71.56 $\pm$ 3.62 & 54.11  $\pm$ 5.33 &  \textbf{77.48 $\pm$ 1.21} \\
5 & \textbf{96.00 $\pm$ 1.63} & 82.54 $\pm$ 0.87 & 77.60 $\pm$  2.21 &  \textbf{91.60 $\pm$ 1.57} & 59.21 $\pm$ 0.99  & 77.76 $\pm$ 0.52\\

10 &  \textbf{98.00 $\pm$ 0.00} & 90.89 $\pm$ 0.22 &  84.33 $\pm$ 2.49 & \textbf{94.90  $\pm$ 1.09} & 66.40 $\pm$ 1.47  & 88.38 $\pm$ 1.40  \\

 & \multicolumn{3}{c}{\textbf{MUTAG}} & \multicolumn{3}{c}{\textbf{Shape}}  \\
\cmidrule(rl){2-4}\cmidrule(rl){5-7}

 & \ourmodel{} & \ourmodel{}-label & Random & \ourmodel{} & \ourmodel{}-label & Random & \\
\midrule
1 & \textbf{71.92 $\pm$ 2.48} & 70.17 $\pm$ 2.48 & 50.87$\pm$ 15.0 &   \textbf{93.33 $\pm$ 4.71} & 60.00  $\pm$ 7.49 & 33.20 $\pm$   4.71\\
5 & 77.19 $\pm$ 4.96 & 57.89 $\pm$ 4.29 & \textbf{80.70 $\pm$  2.40} &    \textbf{96.66 $\pm$ 4.71} & 85.67 $\pm$ 2.45  & 85.39  $\pm$  12.47\\

10 &  \textbf{82.45 $\pm$ 2.48} & 59.65 $\pm$ 8.94  &  75.43 $\pm$ 6.56 &   \textbf{100.00  $\pm$ 0.00} & 88.67 $\pm$ 4.61  & 87.36  $\pm$  4.71  \\

\bottomrule
\end{tabular}
}
\label{tab:label-matching}
\end{table*}

Comparing these results, we can observe that the distribution matching design is effective: disabling this design will greatly deteriorate the performance. 

\subsection{More Qualitative Results}
\label{sec:more-qual}

\noindent\textbf{MUTAG}
This dataset has two classes: ``non-mutagenic'' and ``mutagenic''. As discussed in previous works \cite{debnath1991structure, ying2019gnnexplainer}, Carbon rings along with $NO_2$ chemical groups are known to be mutagenic. And \cite{luo2020parameterized} observe that Carbon rings exist in both mutagen and non-mutagenic graphs, thus are not really discriminative. Our synthesized interpretive graphs are also consistent with these ``ground-truth'' chemical rules. For `mutagenic'' class, we observe two $NO_2$ chemical groups within one interpretative  graph, and one $NO_2$ chemical group and one carbon ring, or multiple carbon rings from a interpretative  graph. For the class of ``non-mutagenic'', we observe that $NO_2$ groups exist much less frequently but other atoms, such as Chlorine, Bromine, and Fluorine, appear more frequently. To visualize the structure more clearly, we limit the max number of nodes to 15 such that we do not have too complicate interpretative  graphs. 

\noindent\textbf{BA-Motif and BA-LRP}
The qualitative results on BA-Motif dataset show that the explanations for all classes successfully identify the discriminative features. For
House-shape class, all the generated graphs have captured such a pattern of house structure, regardless of the complicated base BA graph in the other part of graphs. For the other class with five-node cycle, our generated graphs successfully grasp it from the whole BA-Motif graph. 
In BA-LRP dataset, the first class consists of Barabasi-Albert graphs of growth parameter 1, which means new nodes attached preferably to low degree nodes, while the second class has new nodes attached to Barabasi-Albert graphs preferably to higher degree nodes. Our interpretative  dataset again correctly identify discriminative patterns to differentiate these two classes, which are the tree-shape and ring-shape structures.

% \vskip 0.5em
\noindent\textbf{Shape}
In Table~\ref{tab:qualification}, the generated explanation graphs for all the classes are almost consistent with the desired graph patterns. Note that the difference for interpretative  graphs of Star and Wheel are small. This provides a potential explanation for our post-hoc quantitative results in Table \ref{tab:train-time}, where pre-trained GNN models cannot always distinguish interpretative  graphs of Wheel shape with interpretative  graphs of Star shape.

\begin{table*}[h!]
    \centering
    \begin{tabular}{llcc}
    \toprule
    Dataset & Class & Training Graph Example & Synthesized Interpretation Graph\\
    \midrule
    \multirow{5}{*}{\textbf{BA-Motif}} & House 
        & \begin{minipage}{.2\textwidth}
        \centering
        \includegraphics[width=20mm, height=15mm]{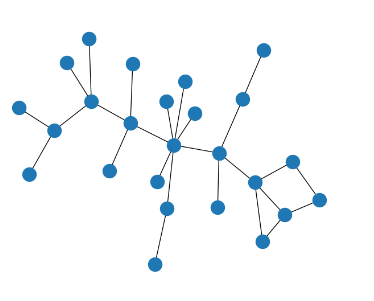}
        \end{minipage} 
        & \begin{minipage}{.3\textwidth}
        \centering
        \includegraphics[width=50mm, height=15mm]{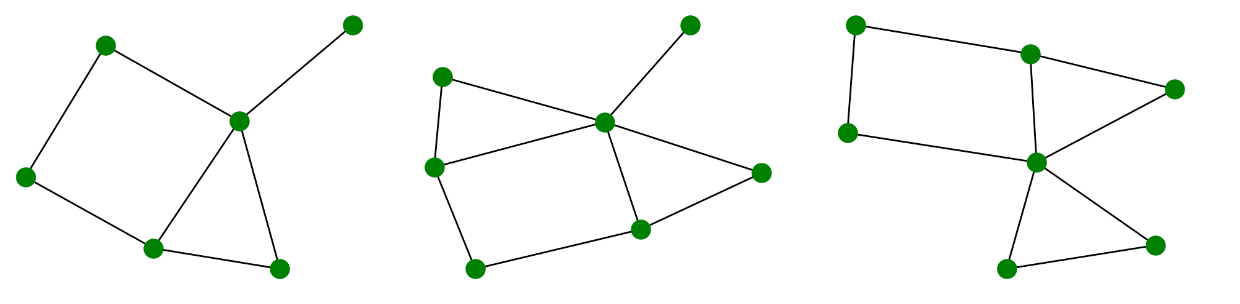}
        \end{minipage} \\
    \cmidrule(rl){2-4}
    & Non-House 
        & \begin{minipage}{.2\textwidth}
        \centering
        \includegraphics[width=20mm, height=15mm]{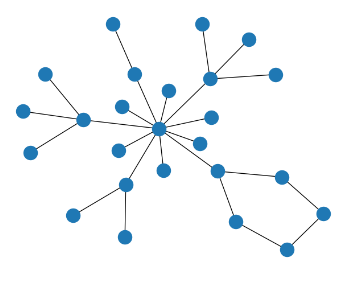}
        \end{minipage}
        & \begin{minipage}{.3\textwidth}
        \centering
        \includegraphics[width=50mm, height=15mm]{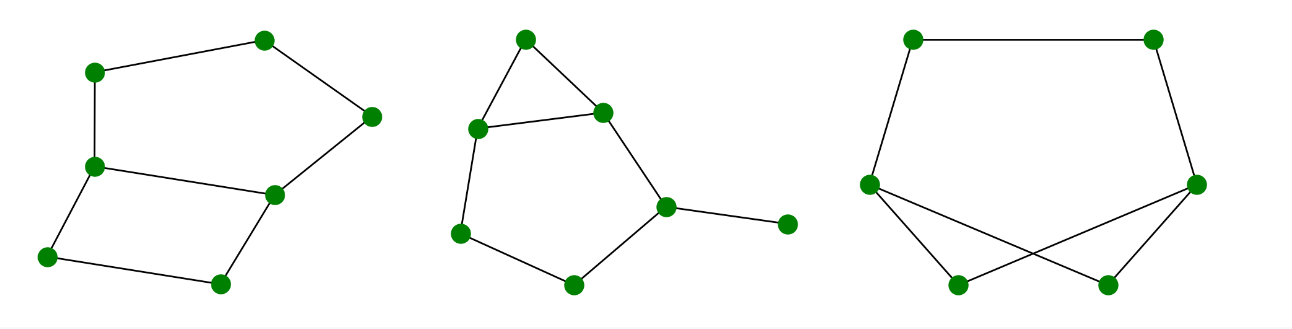}
        \end{minipage} \\
    \midrule
    \multirow{5}{*}{\textbf{BA-LRP}} & Low Degree 
        & \begin{minipage}{.2\textwidth}
        \centering
        \includegraphics[width=20mm, height=15mm]{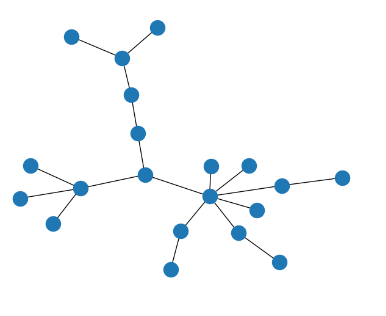}
        \end{minipage} 
        & \begin{minipage}{.3\textwidth}
        \centering
        \includegraphics[width=50mm, height=15mm]{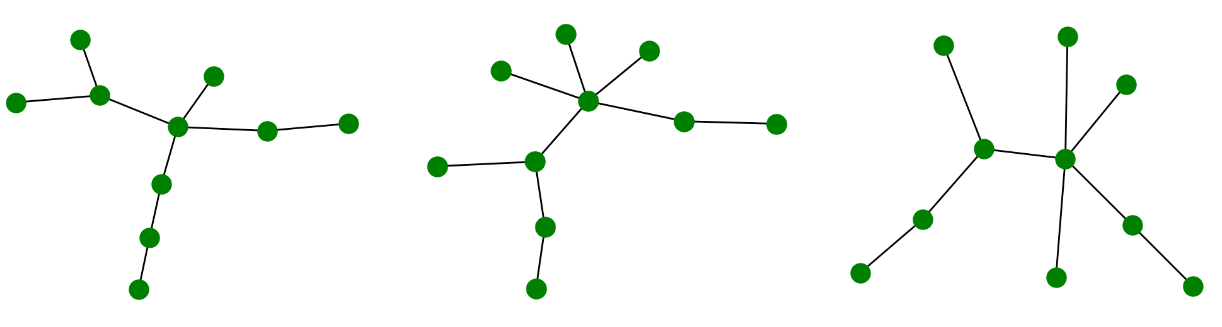}
        \end{minipage} \\
    \cmidrule(rl){2-4}
    & High Degree 
        & \begin{minipage}{.2\textwidth}
        \centering
        \includegraphics[width=20mm, height=15mm]{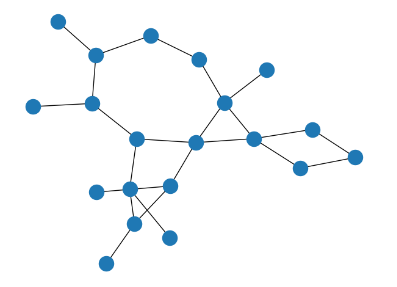}
        \end{minipage}
        & \begin{minipage}{.3\textwidth}
        \centering
        \includegraphics[width=50mm, height=15mm]{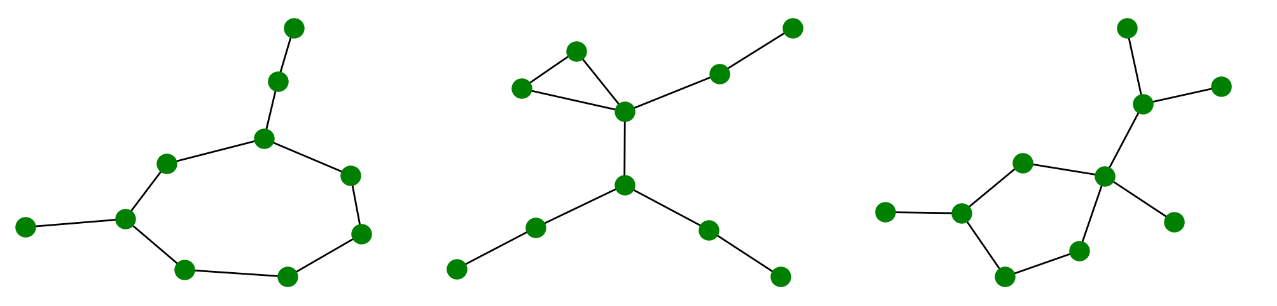}
        \end{minipage} \\
        \midrule
    \multirow{5}{*}{\textbf{MUTAG}} & Mutagenicity
        & \begin{minipage}{.2\textwidth}
        \centering
        \includegraphics[width=20mm, height=15mm]{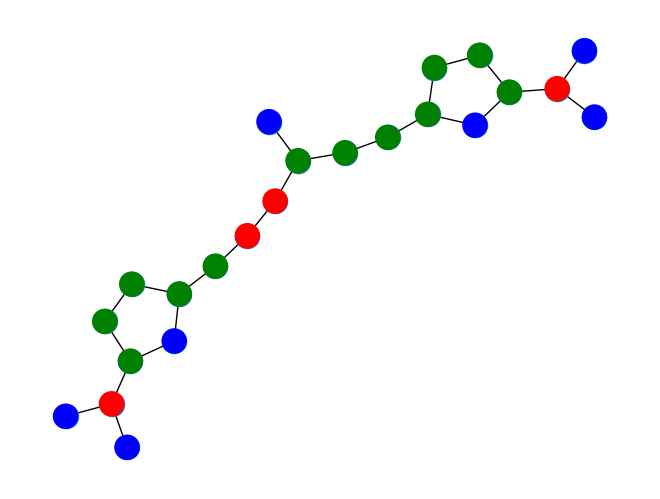}
        \end{minipage} 
        & \begin{minipage}{.3\textwidth}
        \centering
        \includegraphics[width=50mm, height=15mm]{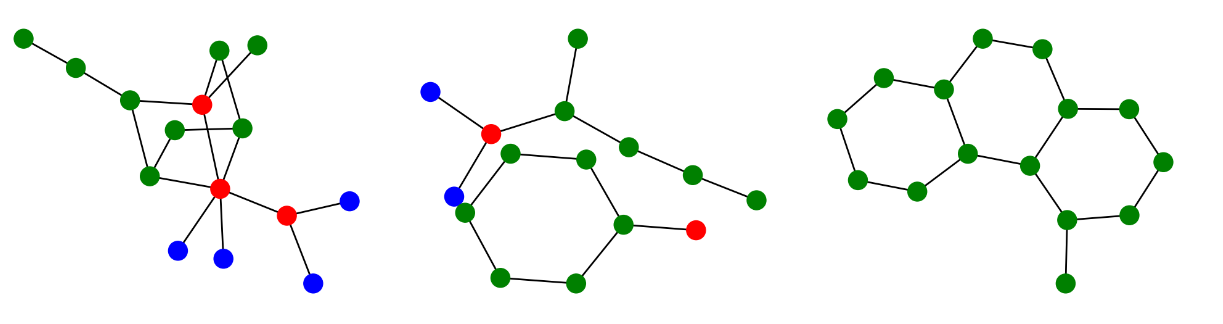}
        \end{minipage} \\
    \cmidrule(rl){2-4}
    & Non-Mutagenicity 
        & \begin{minipage}{.2\textwidth}
        \centering
        \includegraphics[width=20mm, height=15mm]{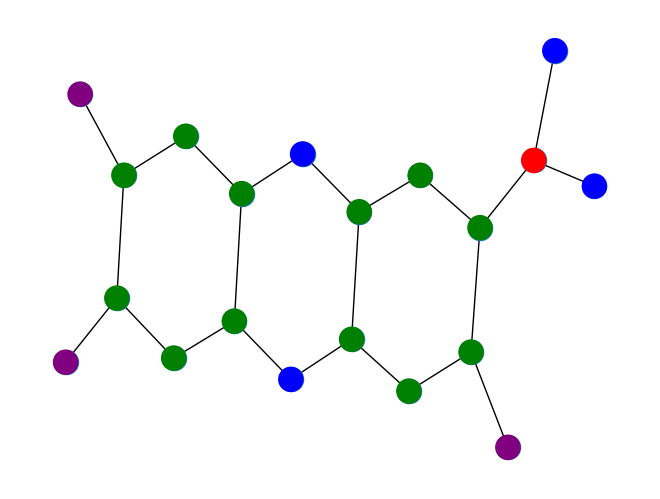}
        \end{minipage}
        & \begin{minipage}{.3\textwidth}
        \centering
        \includegraphics[width=50mm, height=15mm]{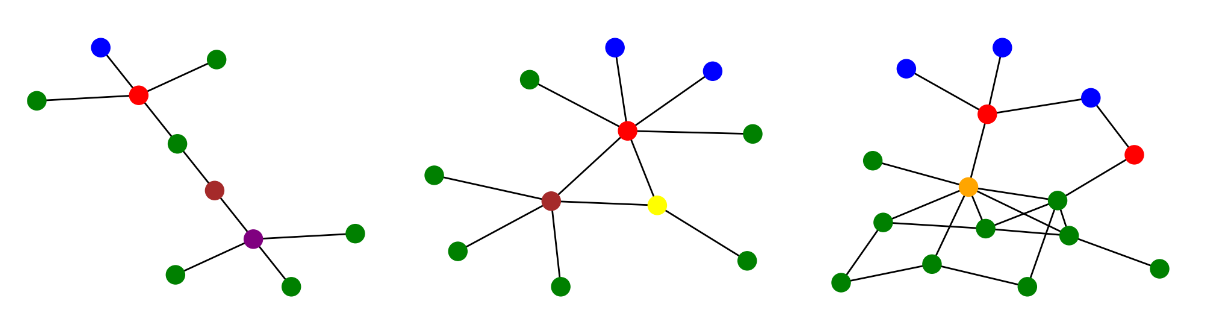}
        \end{minipage} \\
    \midrule
    \multirow{15}{*}{\textbf{Shape}} & Wheel
        & \begin{minipage}{.2\textwidth}
        \centering
        \includegraphics[width=20mm, height=15mm]{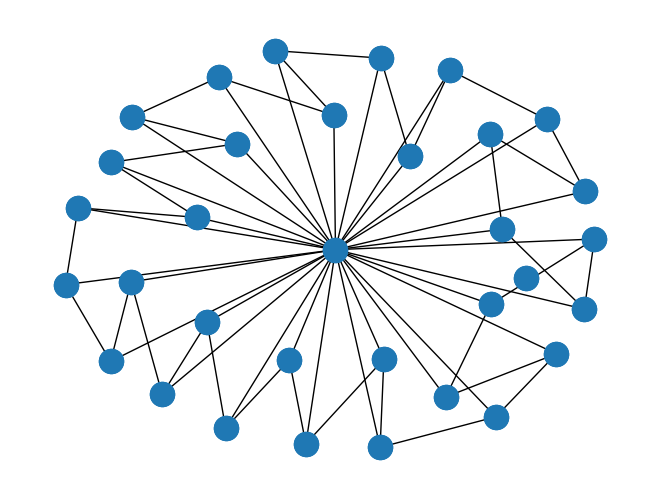}
        \end{minipage} 
        & \begin{minipage}{.3\textwidth}
        \centering
        \includegraphics[width=50mm, height=15mm]{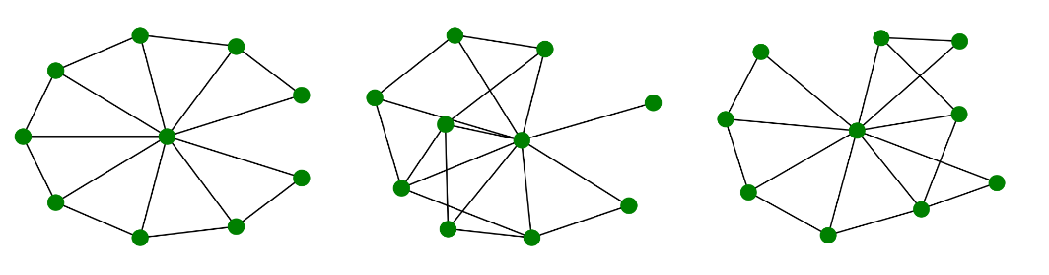}
        \end{minipage} \\
    \cmidrule(rl){2-4}
    & Lollipop
        & \begin{minipage}{.2\textwidth}
        \centering
        \includegraphics[width=20mm, height=15mm]{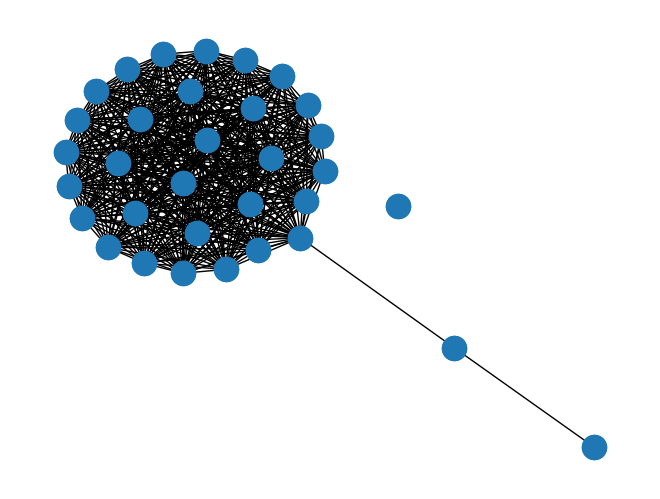}
        \end{minipage}
        & \begin{minipage}{.3\textwidth}
        \centering
        \includegraphics[width=50mm, height=15mm]{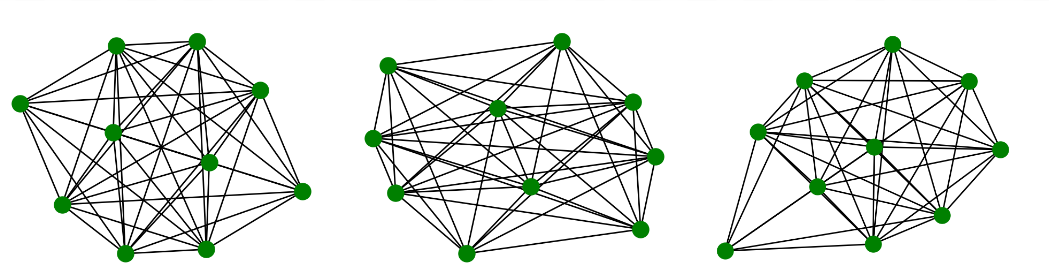}
        \end{minipage} \\
    \cmidrule(rl){2-4}
    & Grid
        & \begin{minipage}{.2\textwidth}
        \centering
        \includegraphics[width=20mm, height=15mm]{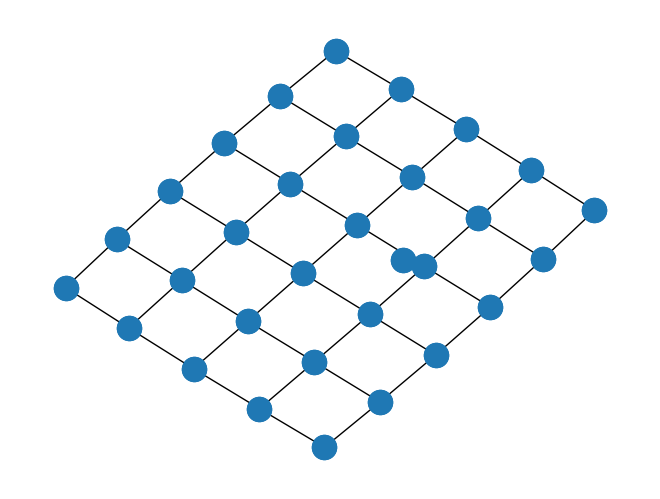}
        \end{minipage}
        & \begin{minipage}{.3\textwidth}
        \centering
        \includegraphics[width=50mm, height=15mm]{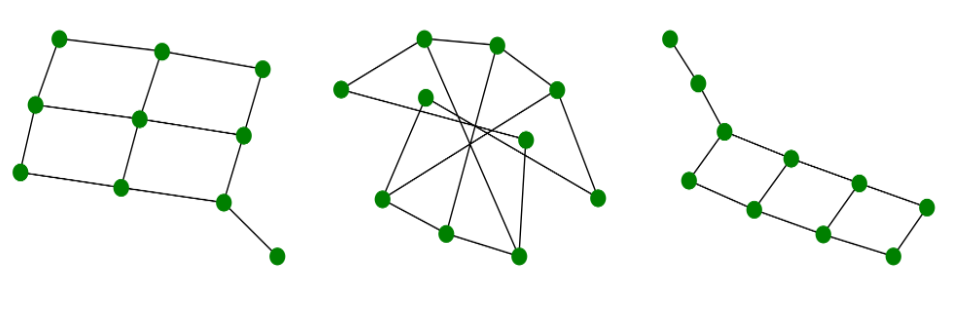}
        \end{minipage} \\
    \cmidrule(rl){2-4}
    & Star
        & \begin{minipage}{.2\textwidth}
        \centering
        \includegraphics[width=20mm, height=15mm]{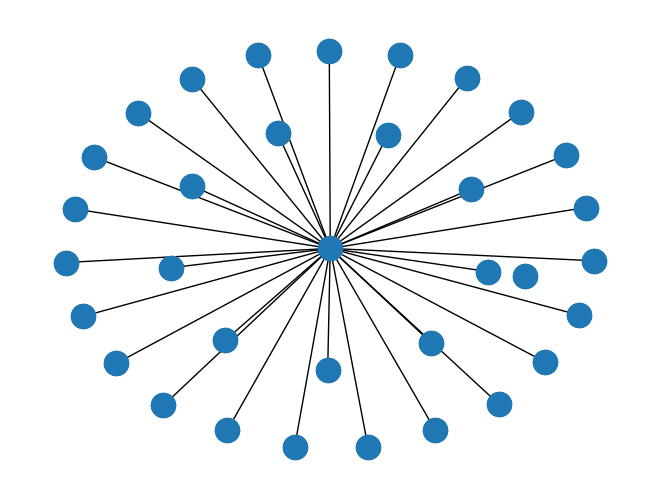}
        \end{minipage}
        & \begin{minipage}{.3\textwidth}
        \centering
        \includegraphics[width=50mm, height=15mm]{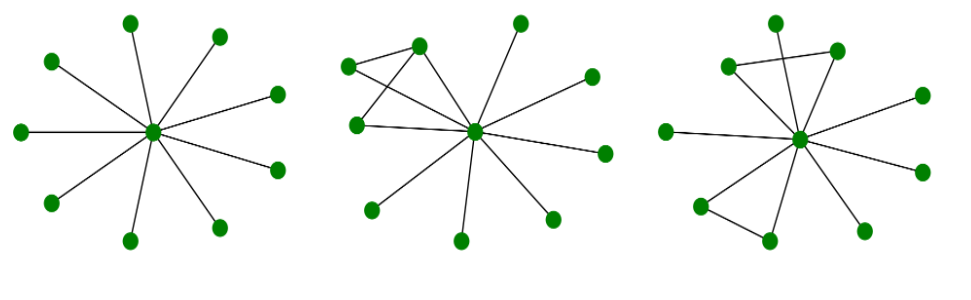}
        \end{minipage} \\    
    % \cmidrule(2)
    \bottomrule 
    \end{tabular}
    \caption{The qualitative results for all datasets. For each class in each dataset, as a reference, the example graph selected from the training data is displayed in the left column, while the generated explanation graphs are in the right column. Different node colors in MUTAG represent different node types.}
    \label{tab:qualification}
\end{table*}
